# Supplementary material for: An Analysis of Model Robustness across Concurrent Distribution Shifts
Source: arXiv:2501.04288 source file (2025-01-08)

**ViT  
pre-training**

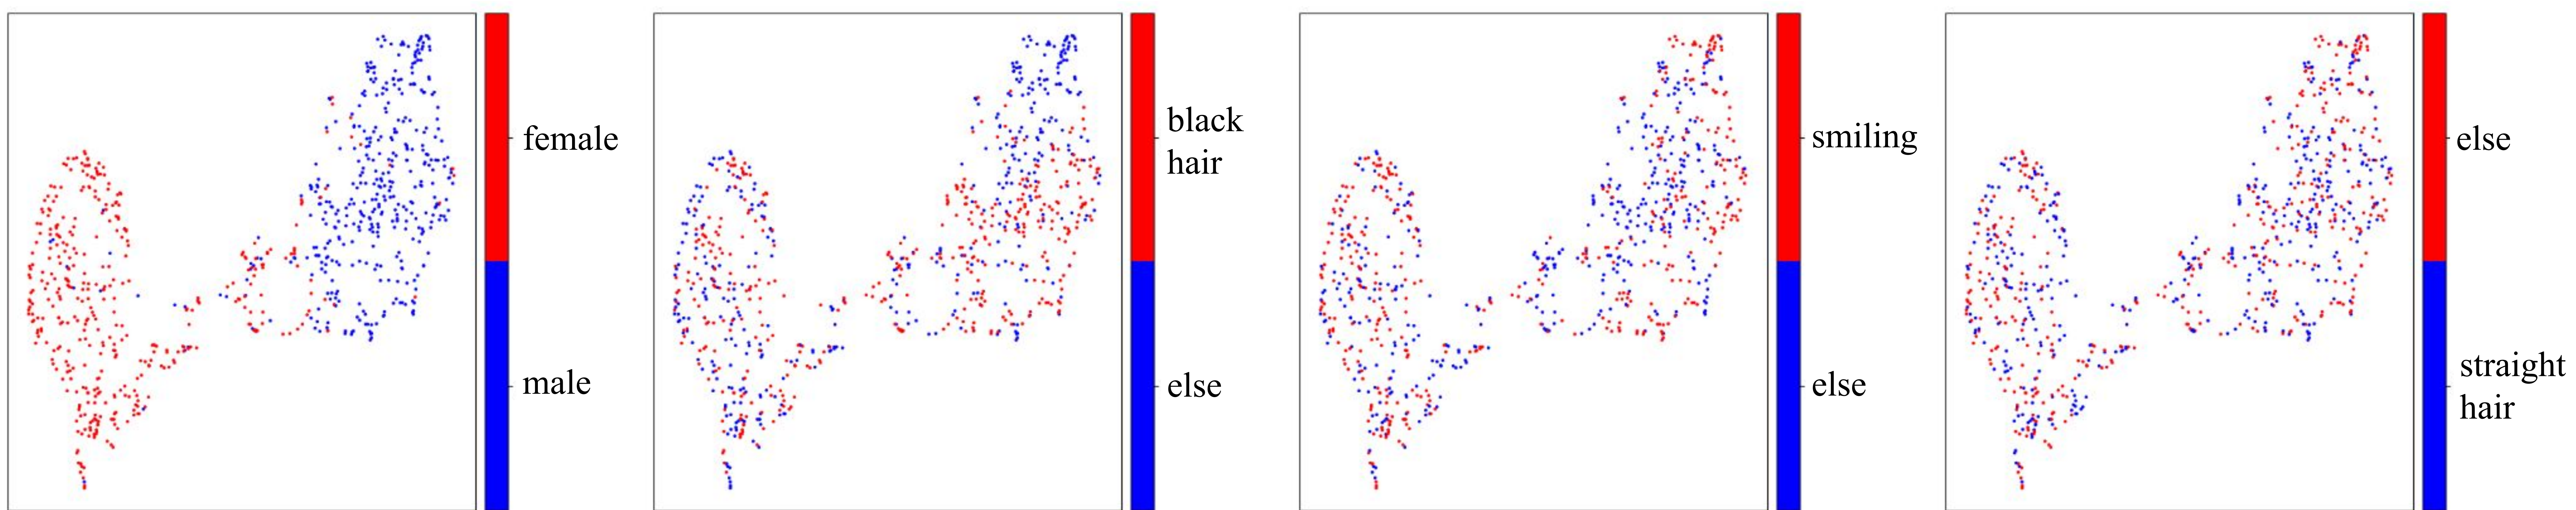

**ViT  
scratch**

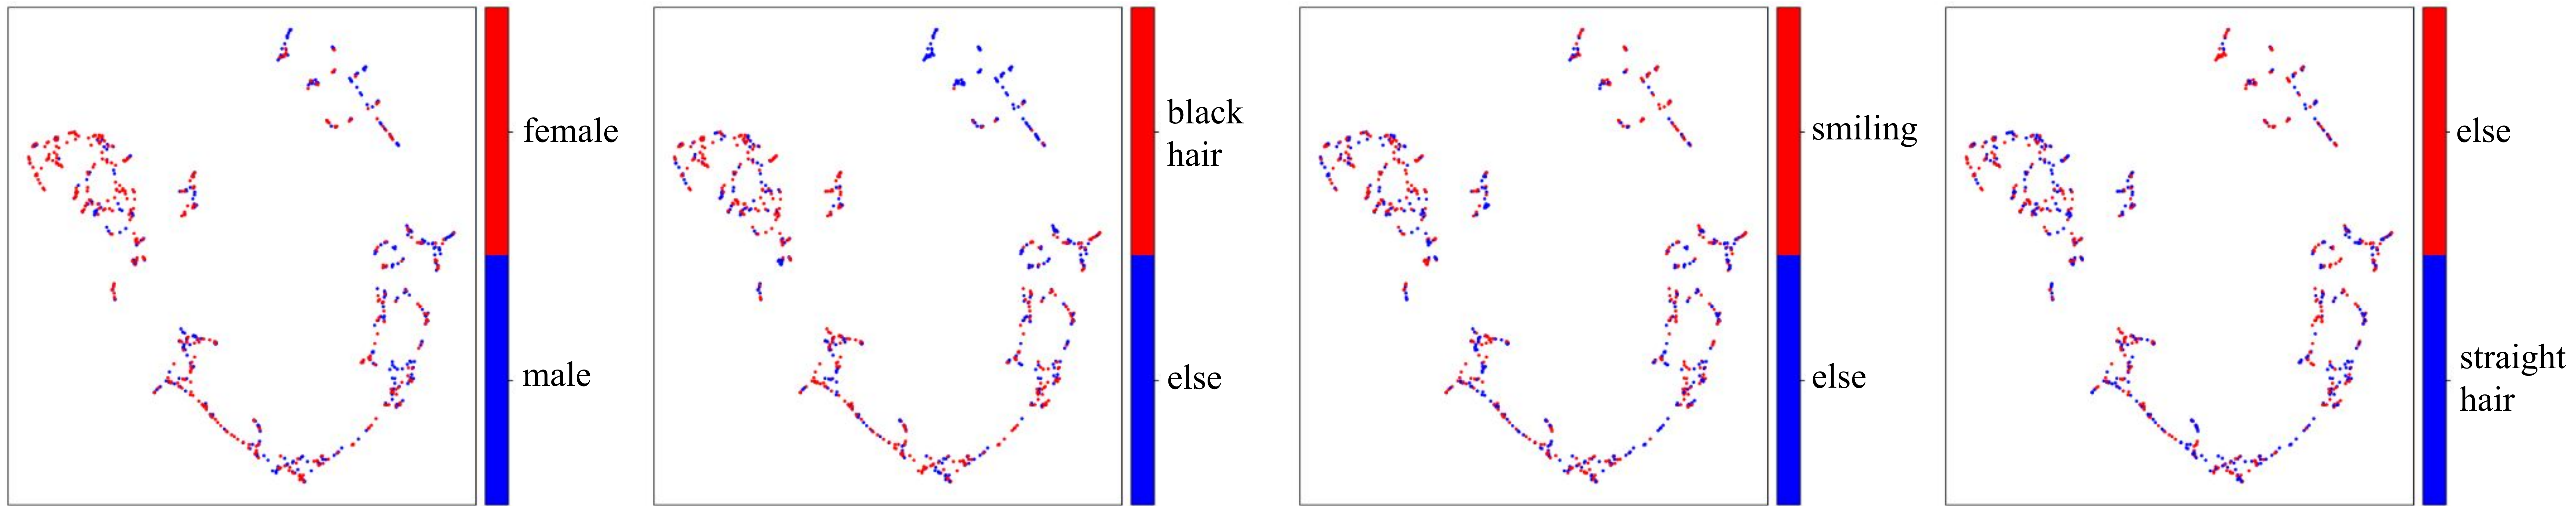



**ImageNet  
augmentation**

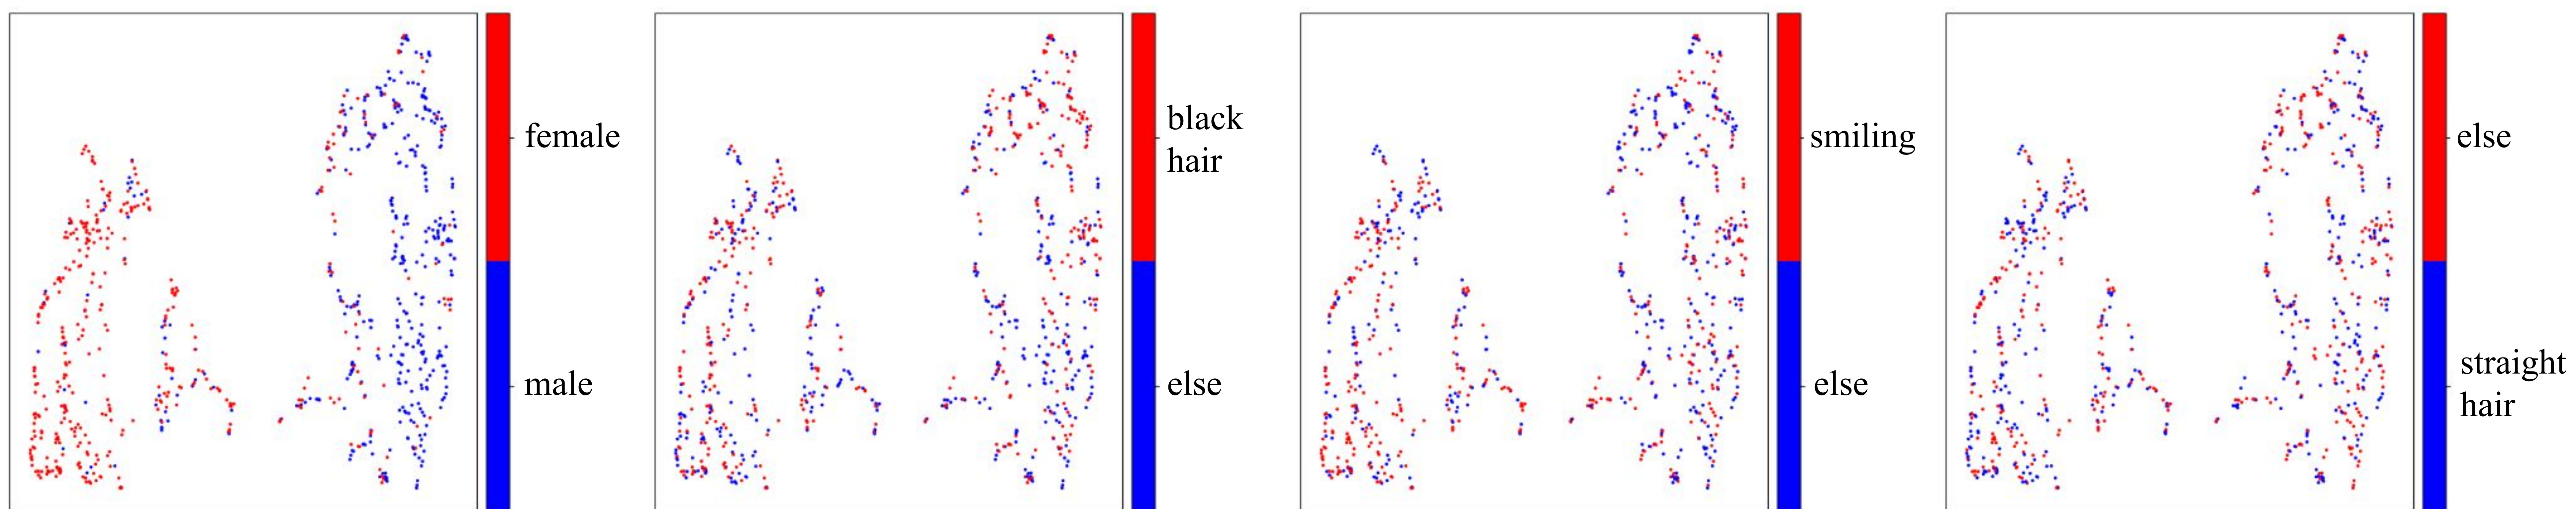

**ViT**

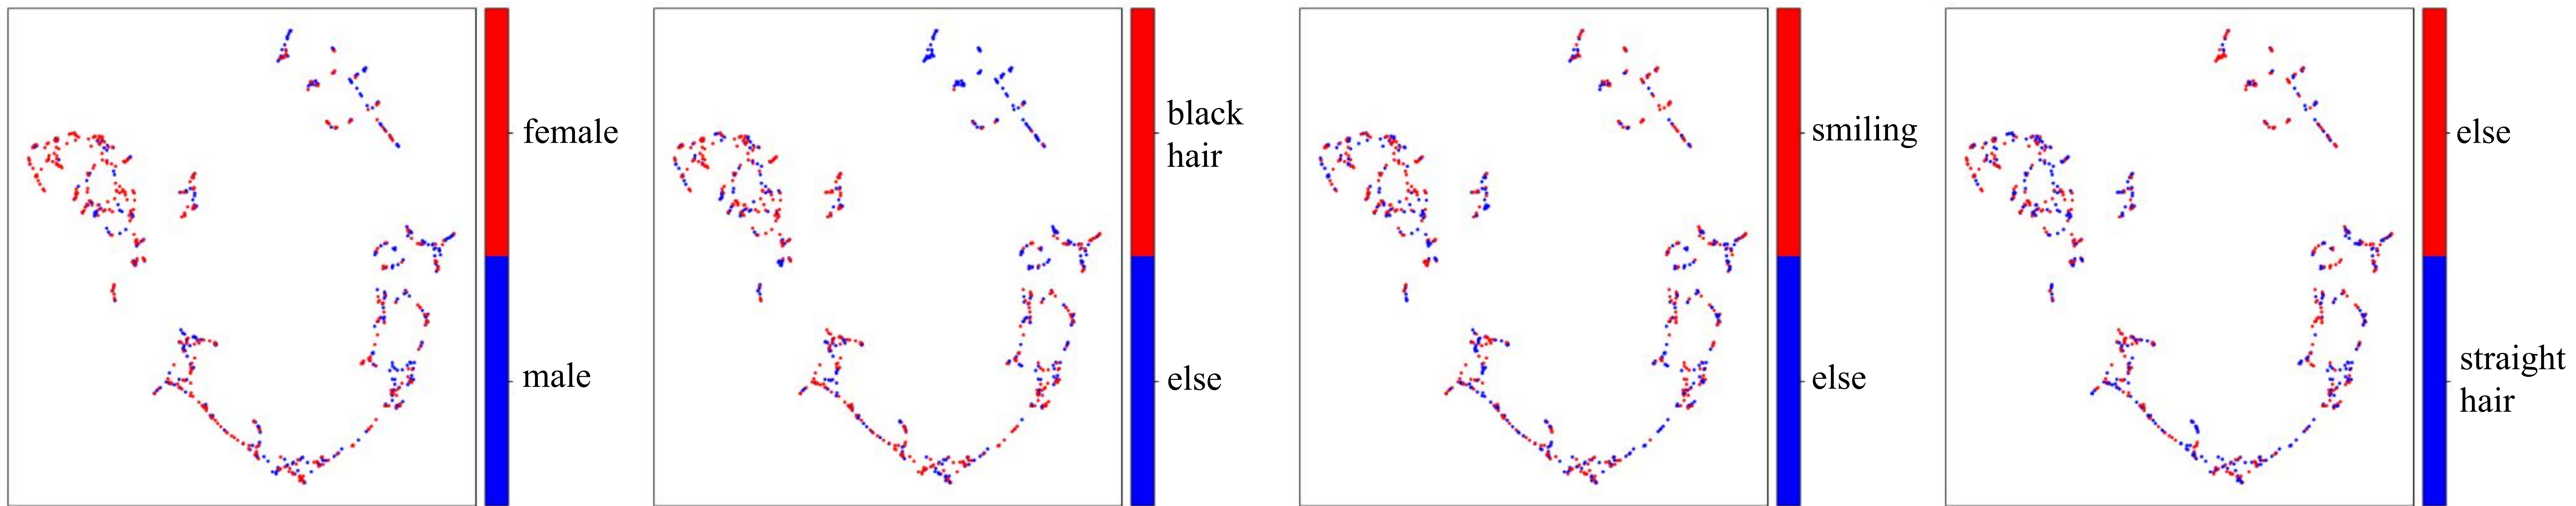



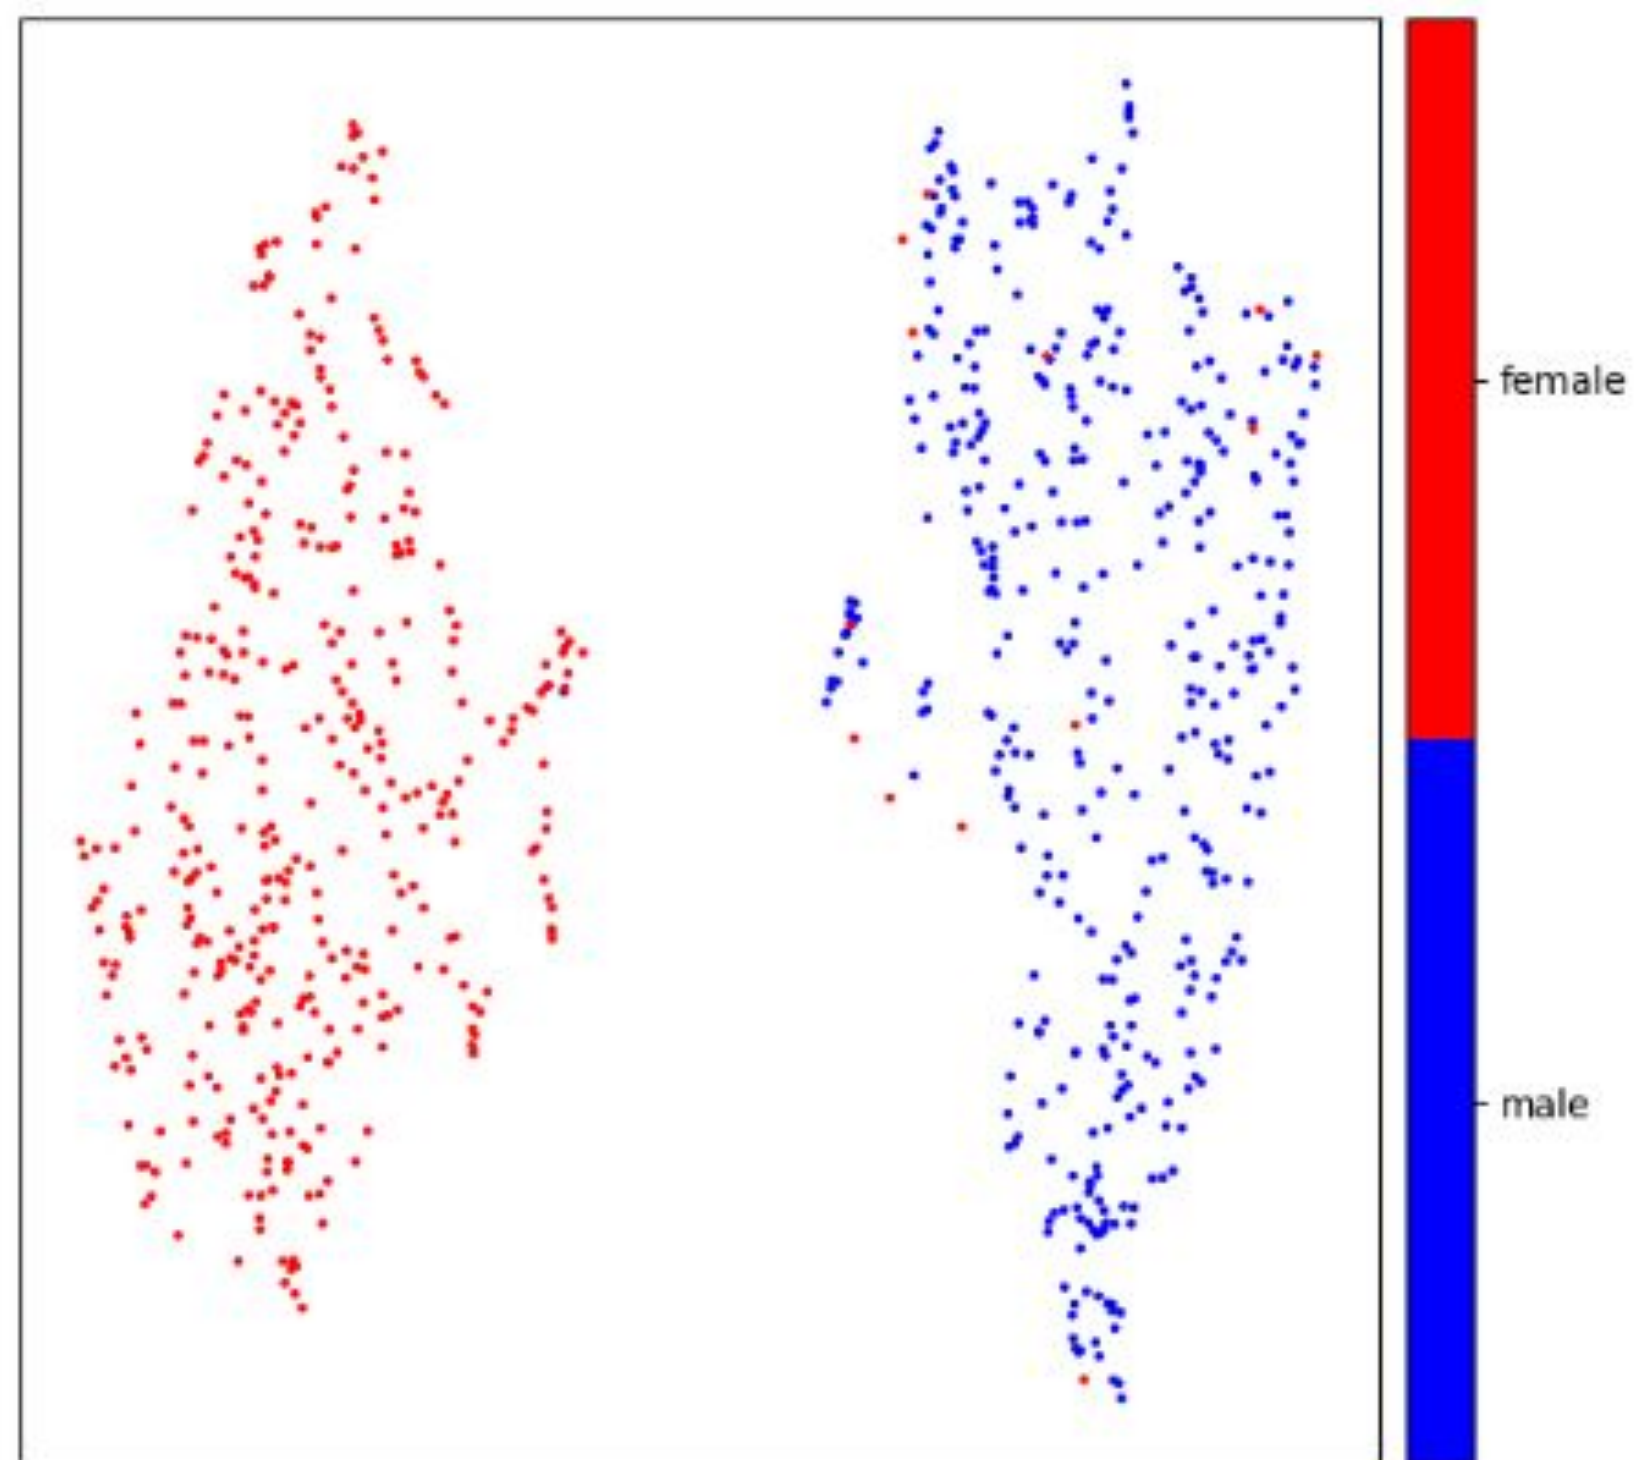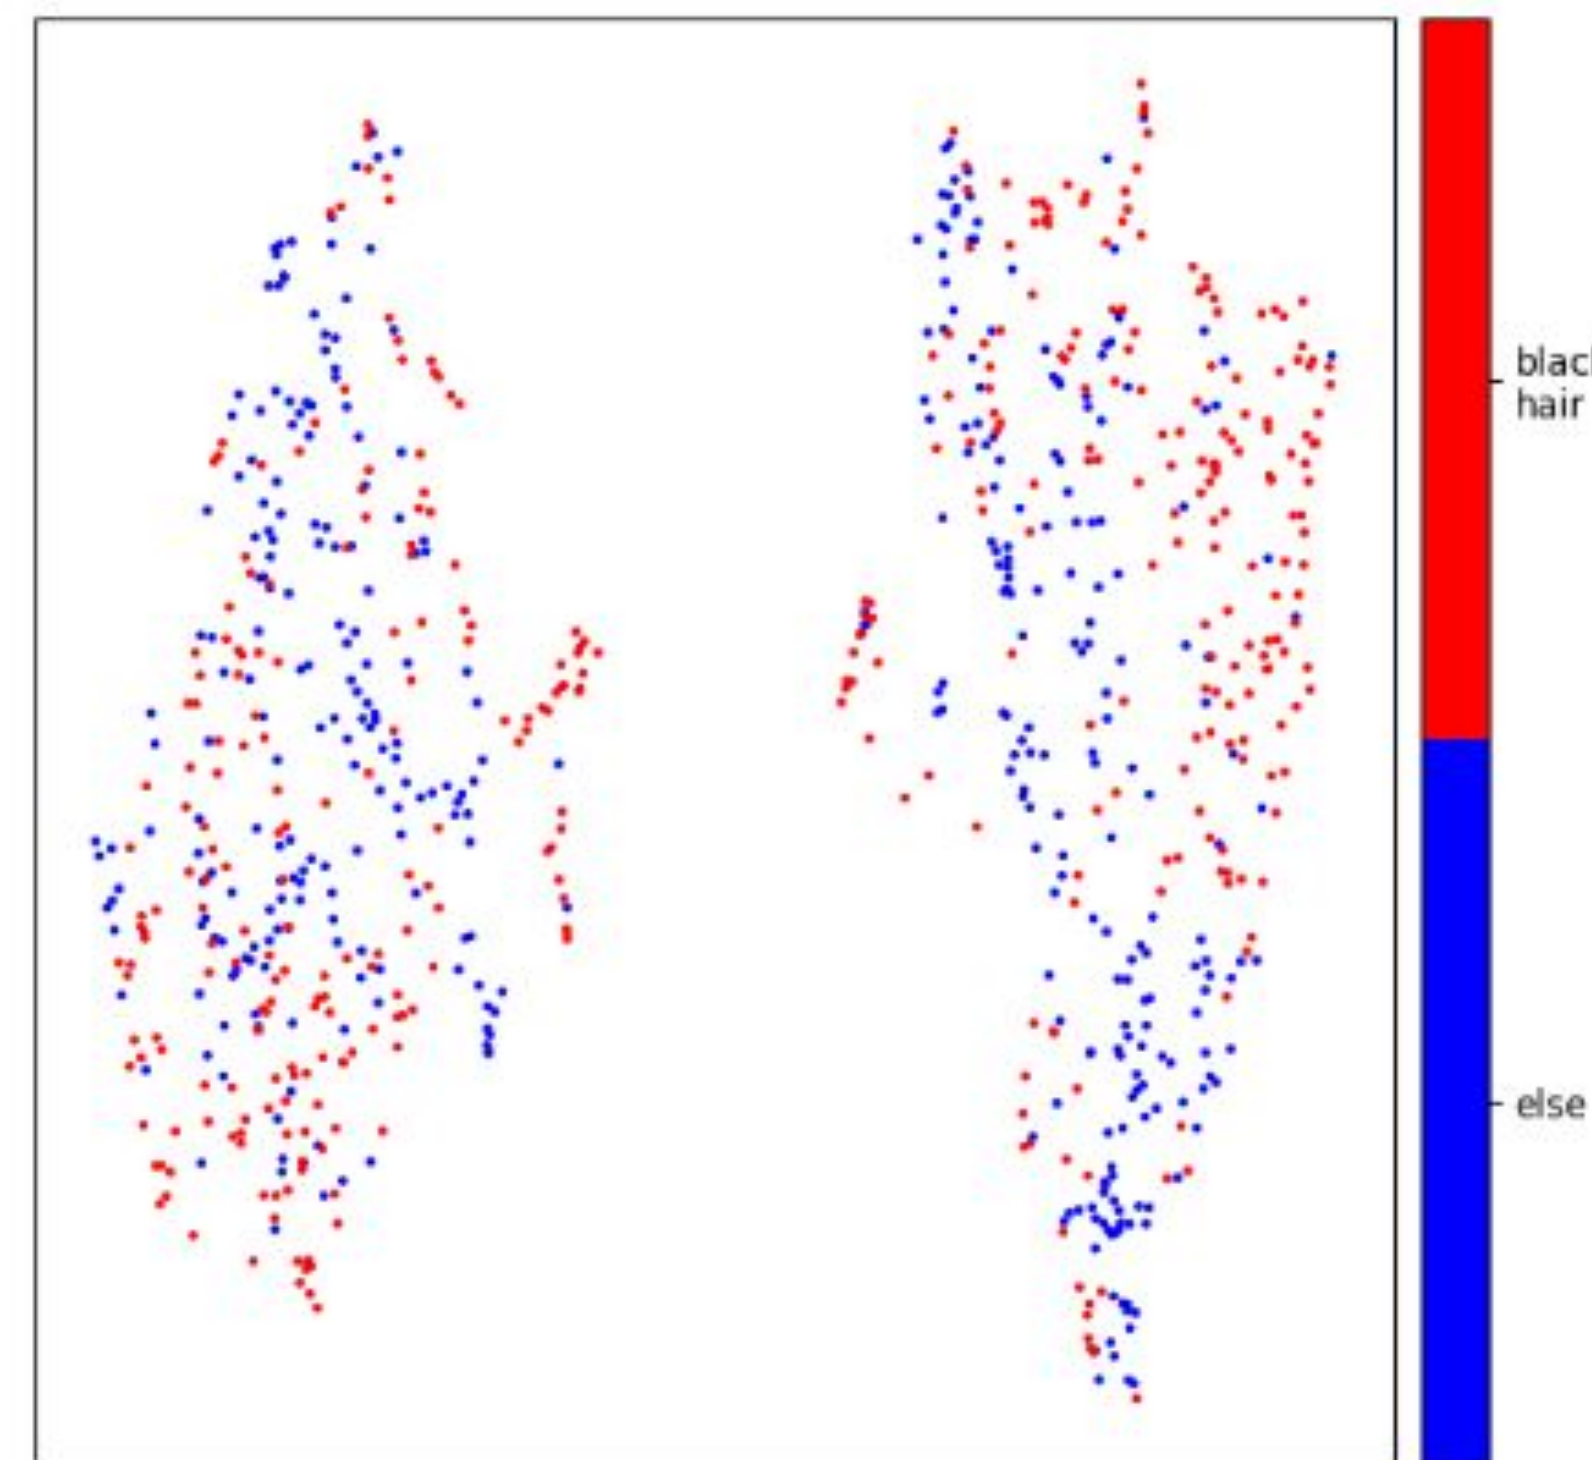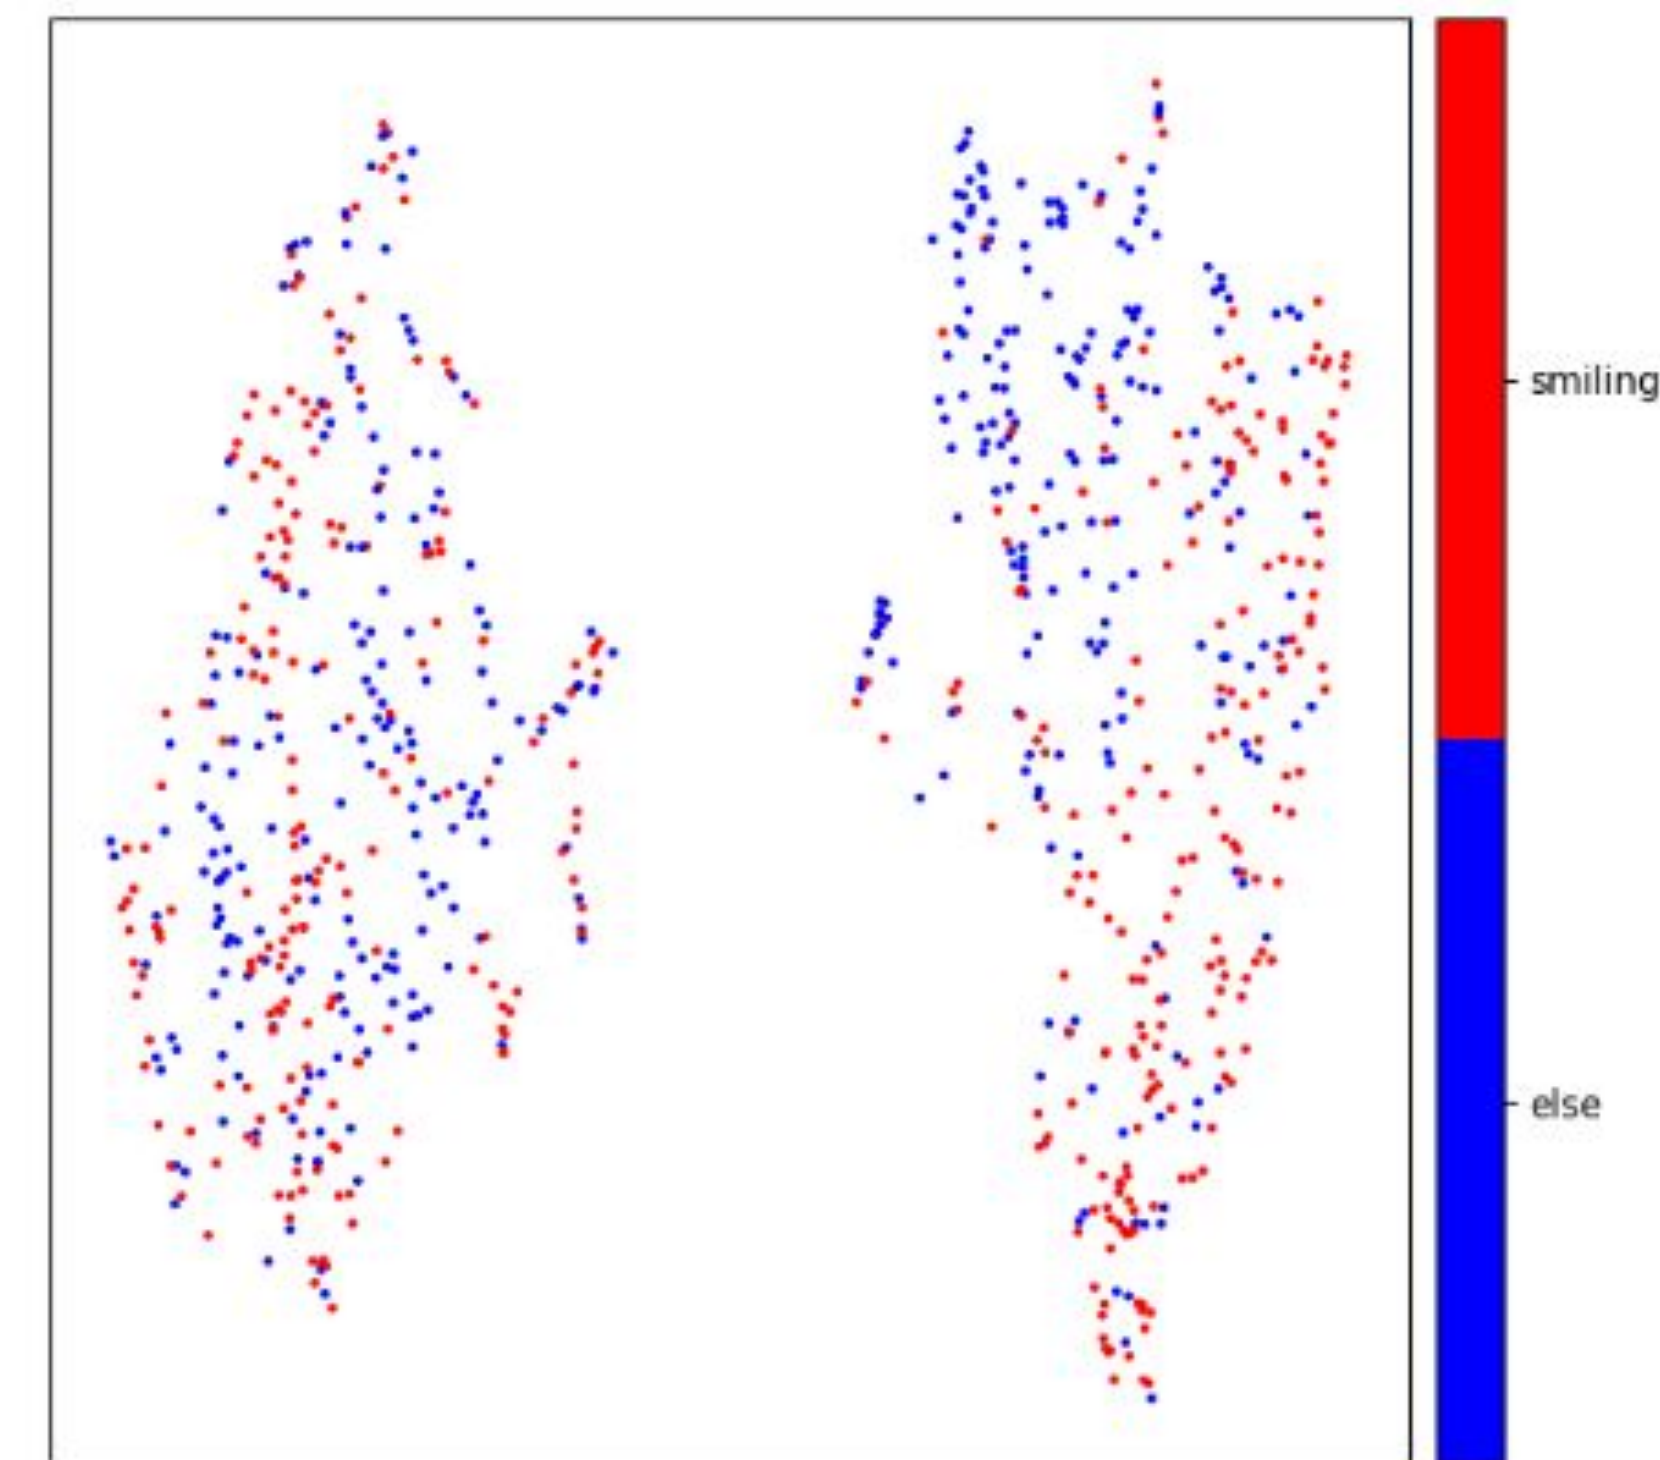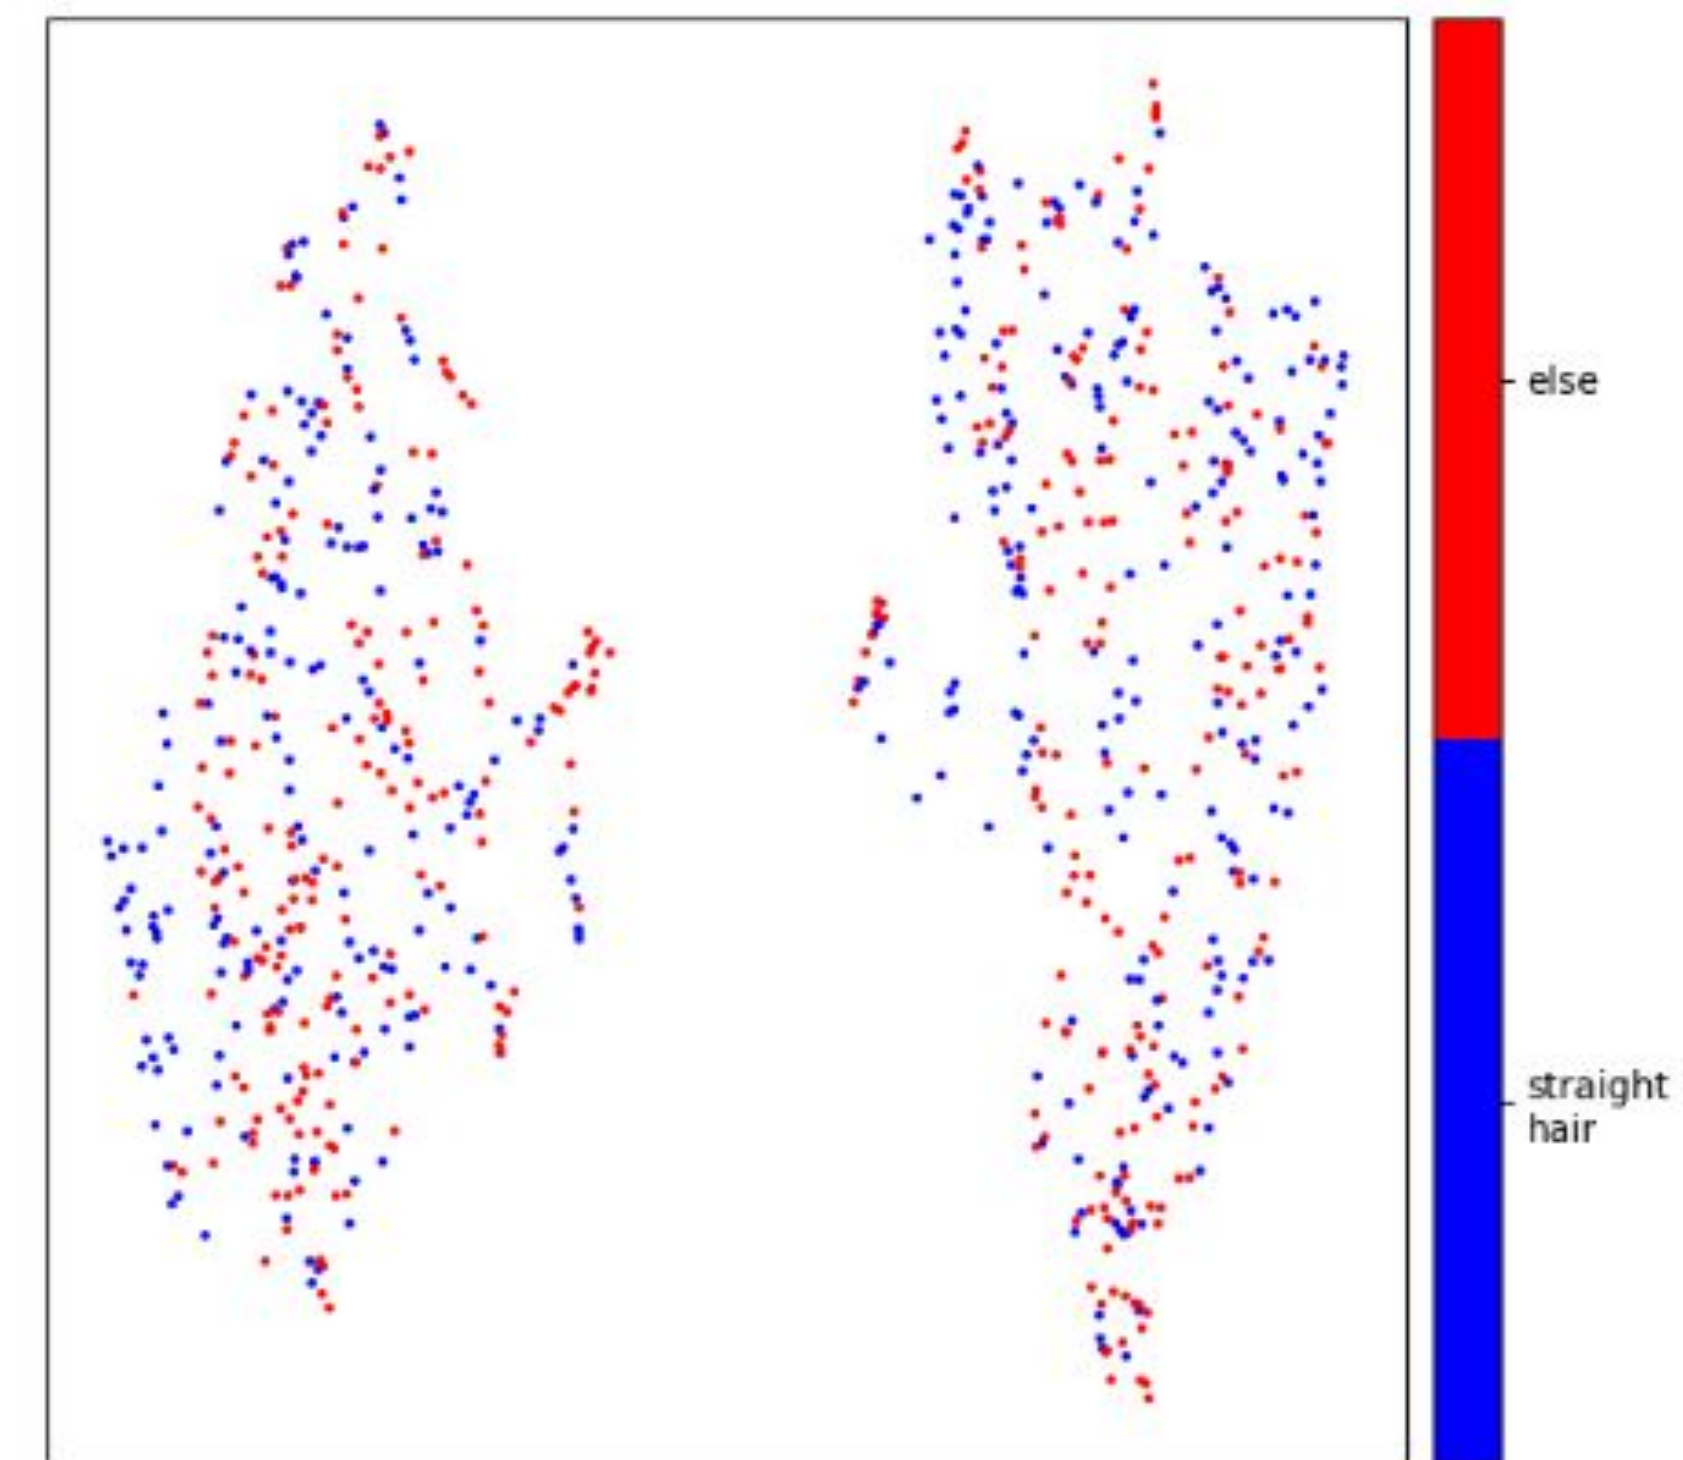

Supplement: Supplementary file 1 [file umap_pretraining.pdf]
